# Supplementary material for: Distribution Estimation under the Infinity Norm
Source: arXiv:2402.08422 source file (2024-02-13)
Supplement: Supplementary file 1 [file Appendix.tex]

\documentclass[a4paper,11pt,oneside]{article}
\usepackage[margin=1in]{geometry}
\usepackage{amsmath, amsthm, amssymb}
\usepackage{hyperref}
\usepackage{mathtools}
\usepackage[round]{natbib}

\hypersetup{
	colorlinks=true,
  linkcolor=red,          %
  citecolor=blue,         %
  filecolor=magenta,      %
  urlcolor=cyan           %
}

\usepackage[utf8]{inputenc} % allow utf-8 input
\usepackage[T1]{fontenc}    % use 8-bit T1 fonts
\usepackage{hyperref}       % hyperlinks
\usepackage{url}            % simple URL typesetting
\usepackage{booktabs}       % professional-quality tables
\usepackage{amsfonts}       % blackboard math symbols
\usepackage{nicefrac}       % compact symbols for 1/2, etc.
\usepackage{microtype}      % microtypography

\usepackage{mathtools}
\usepackage{amsthm, amssymb}
\iffalse
\newtheorem{theorem}{Theorem}[section]
\newtheorem{lemma}{Lemma}[section]
\newtheorem{exercise}{Exercise}[section]
\newtheorem{definition}{Definition}[section]
\newtheorem{proposition}{Proposition}[section]
\newtheorem{property}{Property}[section]
\newtheorem{observation}{Observation}[section]
\newtheorem{note}{Note}[section]
\newtheorem{example}{Exemple}[section]
\newtheorem{question}{Question}[section]
\newtheorem{conjecture}{Conjecture}[section]
\newtheorem{corollary}{Corollary}[section]

\fi
\newcommand{\bepf}{\begin{proof}}
\newcommand{\enpf}{\end{proof}}

\usepackage[ruled,vlined]{algorithm2e}

\usepackage{import}

\usepackage{amsthm}
%\usepackage{algorithm}
%\usepackage[noend]{algpseudocode}
%\floatname{algorithm}{Procedure}
\usepackage{mathtools}
\usepackage{bbm}

\usepackage[ddmmyyyy]{datetime}

\newtheorem{theorem}{Theorem}
\newtheorem{lemma}{Lemma}
\newtheorem{definition}{Definition}
\newtheorem{proposition}{Proposition}
\newtheorem{note}{Note}[section]
\newtheorem{conjecture}{Conjecture}
\newtheorem{corollary}{Corollary}
\newtheorem{remark}{Remark}

%%%%%%%%%% SECTIONS %%%%%%%%%%

\iffalse

\newtheorem{proposition}{Proposition}[section]

\fi

%%%%%%%%%% SET %%%%%%%%%%

%[pred]icate indicator
%\newcommand{\pred}[1]{\boldsymbol{1}\left\{#1\right\}}

%Usual sets

%\newcommand{\F}{\mathbb{F}}

%%%%%%%%%% LINEAR ALGEBRA %%%%%%%%%%

%%%%%%%%%% FUNCTIONS %%%%%%%%%%

%%%%%%%%%% NORMS AND DELIMITERS %%%%%%%%%%

\newcommand{\vertiii}[1]{{\left\vert\kern-0.25ex\left\vert\kern-0.25ex\left\vert #1 
    \right\vert\kern-0.25ex\right\vert\kern-0.25ex\right\vert}}

\usepackage{xcolor}

% TODOs
%\newcommand{\Do}[1]{\todo[color=red!40, inline]{Do: #1}}
%\newcommand{\Ar}[1]{\todo[color=green!40, inline]{Ar: #1}}
%\newcommand{\Ge}[1]{\todo[color=blue!40, inline]{Ge: #1}}
%\newcommand{\Aa}[1]{\todo[color=purple!40, inline]{Aa: #1}}

%\usepackage{todonotes}

%\newcommand{\decr}[1]{\overset{\scalebox{0.4}{\boldsymbol{\phantom{i}_\searrow}\boldsymbol{\phantom{i}_\searrow}}}{#1}}

\newcommand{\beq}{\begin{eqnarray*}}
\newcommand{\eeq}{\end{eqnarray*}}
\newcommand{\beqn}{\begin{eqnarray}}
\newcommand{\eeqn}{\end{eqnarray}}

\usepackage{ifmtarg}
\usepackage{xifthen}% provides \isempty test
\newcommand{\ent}[1][]{%
\ifthenelse{\isempty{#1}}{%
\mathrm{H}
}{
\mathrm{H}^{(#1)}
}}

\newcommand{\loch}[1][]{%
\ifthenelse{\isempty{#1}}{%
\mathrm{h}
}{
\mathrm{h}^{(#1)}
}}

\newcommand{\hide}[1]{}

\usepackage{fancyvrb} % for "\Verb" macro
%Aryeh comment

%Amichai comment

\begin{document}

\section*{Appendix}
\begin{proposition}
Let $n\geq10$ and $\beta=\log(n)$. Then, 
$$f(n)=\frac{\beta^{-\beta} n^2 \left(\frac{n-\beta}{n}\right)^{\beta-n}}{2^\beta-2}\leq
\frac{81}{2}.$$
\end{proposition}
\begin{proof}
    To prove the above, we show that $f(n)$ is decreasing for $n>200$. This means that the maximum of $f(n)$ may be numerically evaluated in the range $n\in\{10,...,200\}$. Finally, we verify that the maximum of $f(n)$ is attained for $n=33$, and is bounded from above by $81/2$ as desired. 
    Let us now show that $f(n)$ is decreasing for $n>200$. Since $f(n)$ is non-negative, it is enough to show that $g(n)=\log f(n)$ is decreasing. Denote
    \begin{align}
    g(n)=-\beta\log \beta+2\log n +(n-\beta)\log(n-\beta)+(n-\beta)\log n -\log(2^\beta-2).
    \end{align}
    Taking the derivative of $g(n)$ we have,
    \begin{align}
        g'(n)=&-\frac{1}{n}(\log \beta+1)+\frac{2}{n}+\left(1-\frac{1}{n}\right)(-\log(n-\beta)-1+\log n) +\frac{n-\beta}{n}-\frac{1}{n}\frac{2^\beta\log 2}{2^\beta-2}=\\\nonumber
        &\frac{1}{n}\left((n-1)\log \frac{n}{n-\beta}-\log \beta -\beta +2 -\frac{2^\beta\log 2}{2^\beta-2}\right)\leq\\\nonumber
        &\frac{1}{n}\left(n\log \frac{n}{n-\beta}-\log \beta -\beta+2 -\log 2\right)\leq
        \frac{1}{n}\left(\frac{n\beta}{n-\beta}-\log \beta -\beta +2 -\log 2\right)=\\\nonumber
        &\frac{1}{n}\left(\frac{\beta^2}{n-\beta}-\log \beta  +2 -\log 2\right)
    \end{align}
    where the first inequality follows from $\log (n /(n-\beta))\geq 1$ and $2^\beta/(2^\beta-2)\geq 1$, while the second inequality is due to Bernoulli Inequality, $(n/(n-\beta))^n\leq \exp(n\beta/(n-\beta))$.  
    Finally, it is easy to show that $\beta^2/(n-\beta)$ is decreasing for $n\geq 10$. This means that $\beta^2/(n-\beta)\leq (\log 10)^2/(10-\log(10))$ and $g'(n)<0$ for $n>200$.
\end{proof}

\end{document}
